# Supplementary material for: A Mechanistic View on Video Generation as World Models: State and Dynamics
Source: arXiv:2601.17067 source file (2026-01-22)
Supplement: Supplementary file 1 [file appendix.tex]

\appendix

\section*{A. Statistics on Visual Recognition VLM Publications}

As shown in Figure 1 (in the main manuscript), we count the number of visual recognition VLM
publications on Google Scholar over the past two years.
Specifically, we consider all the papers that have cited the pioneer VLM study ($i.e.$, CLIP) as potential publications and identify a publication as the visual recognition VLM study if it contains any one of the keywords image classification, object detection, and semantic segmentation.
For the year 2023, we project the total publications based on the number of publications from 1 Jan 2023 to 30 November 2023.

\section*{B. Datasets for Pre-training VLM}

For VLM pre-training, multiple large-scale image-text datasets~\cite{radford2021learning,jia2021scaling,schuhmann2021laion,schuhmann2022laion} were collected from  
the internet.
Compared with traditional crowd-labelled datasets~\cite{deng2009imagenet,cordts2016cityscapes,everingham2010pascal}, the image-text datasets~\cite{schuhmann2021laion,radford2021learning} 
are much larger and cheaper to collect. 
For example, recent image-text datasets are generally at billion scale~\cite{schuhmann2021laion,schuhmann2022laion,chen2022pali}.
Beyond image-text datasets, several studies~\cite{li2022grounded,yu2022coca,yaodetclip,tschannen2022image} utilize auxiliary datasets to provide additional information for better vision-language 
modelling, $e.g.$, GLIP~\cite{li2022grounded} leverages Object365~\cite{shao2019objects365} for extracting region-level features.

\subsection*{B.1. Image-Text Datasets}
\begin{itemize}

    \item \textbf{SBU~\cite{ordonez2011im2text}} contains 1M images collected from the Flicker website, paired with visually relevant captions.
    
    \item \textbf{COCO Caption~\cite{chen2015microsoft}} contains over 330k images from MS COCO~\cite{lin2014microsoft}. It has two versions: COCO Caption c5 with 5 reference captions for 330k images and COCO Caption c40 that provides 40 reference captions for a randomly sampled subset of 5,000 images. 
    
    \item \textbf{YFCC100M~\cite{thomee2016yfcc100m}} is a multimedia dataset containing 99.2M images and 0.8M videos with texts.

    \item \textbf{VG~\cite{krishna2017visual}} provides a multi-perspective understanding of images, $e.g.$, object-level information, scene graphs, and visual question answer pairs. VG contains 108,000 images, each with 50 descriptions.

    \item \textbf{CC3M~\cite{sharma2018conceptual}} is an image captioning dataset which consists of about 3.3M image-text pairs from the web.

    \item \textbf{CC12M~\cite{changpinyo2021conceptual}} is introduced specifically for VLM pre-training. By relaxing the data collection pipeline used in CC3M~\cite{sharma2018conceptual}, CC12M collects less precise but a much larger size of data, $i.e.$, 12M image-text pairs.
    
    \item \textbf{LR~\cite{pont2020connecting}} is an image captioning dataset with local multi-modal annotations, where every word is localized in the image with a mouse trace segment. It contains 848,749 images with 873,107 captions.
    
    \item \textbf{WIT~\cite{srinivasan2021wit}} is a large multi-modal multilingual dataset collected from Wikipedia, which consists of 37.6M image-text pairs across 108 languages.

    \item \textbf{Red Caps~\cite{desai2021redcaps}} is an image-text dataset collected from social media Reddit, which contains 12M image-text pairs covering various objects and scenes.

    \item \textbf{LAION400M~\cite{schuhmann2021laion}:} LAION400M consists of 400M image-text pairs filtered by CLIP~\cite{radford2021learning}, which also provides the data embeddings and kNN indices.
    
    \item \textbf{LAION5B~\cite{schuhmann2022laion}} contains over 5.8B image-text pairs, which consists of three parts: 2.32B English image-text pairs, 2.26B multilingual image-text pairs and 1.27B pairs without specific language.

    \item \textbf{WuKong~\cite{gu2022wukong}} is a large-scale Chinese multi-modal dataset, which contains 100M Chinese image-text pairs collected from the web.

    \item \textbf{CLIP~\cite{radford2021learning}} is a large-scale web image-text dataset, which contains 400M image-text pairs collected from a variety of publicly available sources on the internet.
    
    \item \textbf{ALIGN~\cite{jia2021scaling}} is an image-text dataset, which contains 1.8B noisy image-text pairs covering board concepts.

    \item \textbf{FILIP~\cite{yao2021filip}} is a large-scale image-text dataset with 300M image-text pairs collected from the internet.

    \item \textbf{WebLI~\cite{chen2022pali}} is a multilingual image-text dataset collected from the web, which comprises 10B images with 12B corresponding texts across 109 languages.
\end{itemize}

\subsection*{B.2. Auxiliary Datasets}

\begin{itemize}
    \item \textbf{JFT3B~\cite{zhai2022scaling}} contains nearly 3B images annotated with a noisy class hierarchy of around 30k labels.

    \item \textbf{C4~\cite{raffel2020exploring}} is a collection of about 750GB English text sourced from the public Common Crawl web scrape.

    \item \textbf{Object365~\cite{shao2019objects365}} is an object detection dataset with 365 categories, 638K images, and $\sim$10M bounding boxes.

    \item \textbf{Gold-G~\cite{kamath2021mdetr}} is an object-phrase dataset for object detection, which includes 0.8M human-annotated visual grounding data curated by~\cite{kamath2021mdetr}.

\end{itemize}

\section*{C. Datasets for Evaluation}

Many visual recognition datasets have been adopted for VLM evaluations as shown in Table 2 (in the main manuscript), including $27$ image classification datasets, $4$ object detection datasets, $4$ semantic segmentation datasets, $2$ image-text retrieval datasets, and $3$ action recognition datasets.
Please find the details of each dataset below.

\subsection*{C.1. Datasets for Image Classification}

\begin{itemize}
    \item \textbf{Food-101~\cite{bossard2014food}} is a real-world food dataset for fine-grained recognition. The dataset consists of 101,000 images, covering 101 classes.  
    Specifically, every class contains 250 cleaned test samples and 750 purposely uncleaned training samples. 
    
    \item \textbf{CIFAR-10~\cite{krizhevsky2009learning}} contains a set of small images, which is commonly used for image classification tasks. This dataset includes 60000 images with a size of 32 by 32, annotated with ten categories. This dataset has been divided into 5000 training samples and 1000 testing samples per class. 
    
     \item \textbf{CIFAR-100~\cite{krizhevsky2009learning}} is almost the same as CIFAR10, except that CIFAR-100 instead contains 60000 samples with 100 categories that have been grouped into twenty super-categories.

    \item \textbf{Birdsnap~\cite{berg2014birdsnap}} is a fine-grained classification dataset collected from Flicker. There are 49,829 images belonging to 500 bird species, including 47,386 training images and 2433 testing images. In this dataset, every image has been labelled with a bounding box, the coordinates of 17 parts, and auxiliary attribute annotations like male, female, immature, etc.

    \item \textbf{SUN397~\cite{xiao2010sun}} is proposed for scene recognition and contains 39700 images covering 397 well-sampled categories. The scene classification performance by humans is provided as the reference for the comparisons with computational methods.

    \item \textbf{Stanford Cars~\cite{krause2013collecting}} is designed for fine-grained recognition, containing 16185 images covering 196 categories. This dataset has been divided into 8,144 training samples and 8,041 testing samples.

    \item \textbf{FGVC Aircraft~\cite{maji2013fine}} includes 10K samples spanning 100 aircraft model variants. Every sample is labeled with a tight bounding box and a hierarchical category annotation. This dataset has been equally separated into training, validation, and test subsets, where every subset contains 33 or 34 images per variant. 

    \item \textbf{PASCAL VOC 2007 Classification~\cite{everingham2010pascal}} is the widely-used dataset for various visual recognition tasks like detection, segmentation, and classification. There are 9963 samples covering 20 classes, including 5011 training images and 4952 testing images. Every sample in PASCAL VOC 2007 contains pixel-wise labels, object-level labels with object box, and category labels.

    \item \textbf{Describable Textures~\cite{cimpoi2014describing} (DTD)} is a collection of textural images for image recognition. This dataset includes 5640 samples with forty-seven categories, which have been equally separated into training, validation, and test subsets, where each subset contains 40 images per class. For each image, the main category and a list of the joint attributes are provided.

    \item \textbf{Oxford-IIIT PETS~\cite{parkhi2012cats}} includes 7,349 cat and dog images with thirty-seven different breeds, in which twenty-five are dog breeds, and twelve are cat breeds. These samples are separated into the training subset with around 1850 samples, the validation subset with about 1850 samples, and the testing subset with approximately 3700 samples.
    Every sample has been annotated with a breed annotation, a pixel-wise annotation that marks the body, and a rectangle box for locating the head.

    \item \textbf{Caltech-101~\cite{fei2004learning}} consists of 9145 images belonging to 101 classes. Every category includes 40-80 images. For each image, the dataset provides an annotation to segment the foreground object.

    \item \textbf{Oxford 102 Folwers~\cite{nilsback2008automated}} is proposed for fine-grained image classification. This dataset contains 8189 flower images that belong to 102 species. Each category contains 40-200 samples, including the flower captured under various sizes and illumination environments. Besides, this dataset also contains pixel-wise annotations.
    
   \item \textbf{Facial Emotion Recognition 2013~\cite{goodfellow2013challenges}} is collected by requesting images associated with 184 key emotional terms from Google. The dataset contains 35,887 grayscale images with a resolution of 48x48 pixels and with 7 types of emotions.

    \item \textbf{STL-10~\cite{coates2011analysis}} is a type of classification benchmark for researching on unsupervised and self-taught training. It includes 10 categories and an unsupervised training subset with 100K samples, a supervised training subset with 5K samples, and a testing subset with 8K samples.

    \item \textbf{EuroSAT~\cite{helber2019eurosat}} is a set of satellite images used to benchmark the land use and land cover recognition tasks. It covers thirteen frequency bands with ten categories of 27K annotated and geo-referenced samples. Two datasets are provided, including the RGB image dataset and the multi-spectral image dataset.

    \item \textbf{RESISC45~\cite{cheng2017remote}} has been proposed to benchmark Remote Sensing Image Scene Classification (RESISC). This dataset includes 31,500 samples with the image size of 256 by 256 and forty-five scene categories, every category containing 700 samples. 
    Besides, RESISC45 covers a wide range of spatial resolutions from 20cm to over 30m per pixel.
    
    \item \textbf{GTSRB~\cite{stallkamp2011german}} is a dataset for traffic signs classification, containing 50,000 images taken from various street scenes in Germany. It is classified into 43 categories, including a training subset with 39,209 samples and a testing subset with 12,630 samples.

    \item \textbf{Country211~\cite{radford2021learning}} is an image classification dataset for geolocation evaluation, which is a subset of the YFCC100M dataset. For each country, there are one hundred and fifty train samples, fifty validation samples, and one hundred test samples.

    \item \textbf{PatchCamelyon~\cite{veeling2018rotation}} 
    includes 327,680 RGB images with a size of 96 by 96 from Camelyon16, with a training subset with 75\% samples, a validation subset with 12.5\% samples, and a testing subset with 12.5\% samples. 
    Every sample has been labelled with a binary annotation showing if it contains the metastatic tissue.

    \item \textbf{Hateful Memes~\cite{kiela2020hateful}} has been proposed for hateful meme classification ($i.e.$, image with text) created by Facebook AI. It includes over 10k memes annotated with either the hateful label or the non-hateful label.

    \item \textbf{Rendered SST2~\cite{radford2021learning}} has been proposed for benchmarking optical character recognition. It includes 2 categories (the categories of positives and negatives). This dataset has been separated into 3 subsets: a training subset with 6920 samples, a validation subset with 872 samples, and a test subset with 1821 samples.

    \item \textbf{ImageNet-1k~\cite{deng2009imagenet}} includes about 1.2M samples that are uniformly distributed across the one thousand categories. The category annotation of ImageNet-1k follows WordNet hierarchy, and every sample is annotated with one category label. 
    Besides, ImageNet-1k is one of the most popular image classification benchmarks.

    \item \textbf{CLEVR Counts~\cite{johnson2017clevr}} is a subset of the CLEVR dataset, which is designed for visual question answering to evaluate the ability to perform visual reasoning. The counting tasks include 2000 training samples and 500 test samples. 

    \item \textbf{SVHN~\cite{netzer2011reading}} is a dataset for recognizing digits and numbers in real-world images, which are collected from Google Street View images. It consists of about 600,000 images, and all digits are cropped from the images and resized to a fixed resolution of 32x32 pixels.

    \item \textbf{IIIT5k~\cite{mishra2012scene}} contains 5,000 cropped word images collected from Google image search by using search keywords such as signboards, house name plates, and movie posters, etc.
    The dataset is split into two parts, $i.e.$, 2,000 word images for training and 3,000 word images for validation, respectively.

    \item \textbf{Rendered SST2~\cite{socher2013recursive}} is a sentiment classification dataset which consists of two sentiment categories, $i.e.$, negative and positive.
    The sentences in the dataset are extracted from the Stanford Sentiment Treebank dataset.

\end{itemize}

\subsection*{C.2. Datasets for Action Recognition}

\begin{itemize}

    \item \textbf{UCF101~\cite{soomro2012ucf101}} has been proposed for benchmarking human action recognition with videos.    
    It includes about 13k video clips of 101 actions, which are collected from YouTube. 
    The video clips in the dataset have a resolution of 320x240 pixels and a frame rate of 25 FPS.

    \item \textbf{Kinetics700~\cite{carreira2019short}} is a video dataset for recognizing human action. 
    It consists of about 65,000 video clips with 700 human actions, where each action category has more than 700 video clips lasting around 10 seconds.

    \item \textbf{RareAct\cite{miech2020rareact}} is a video dataset designed for identifying rare actions such as ``Unplug Oven'' and ``fry phone''. This dataset aims to evaluate action recognition models on unlikely combinations of common action verbs and object nouns.
    It contains 122 human actions, where the verbs and object nouns in actions are rarely co-occurring together in HowTo100M.

\end{itemize}

\subsection*{C.3. Datasets for Semantic Segmentation}

\begin{itemize}

    \item \textbf{ADE20k~\cite{zhou2017scene}} is a semantic segmentation dataset that consists of 150 classes. It consists of a training subset with 25,574 samples and a validation subset with 2,000 samples.

    \item \textbf{PASCAL VOC 2012 Segmentation~\cite{everingham2010pascal}} contains 20 categories including vehicles, household and animals. This dataset includes a training subset with 1,464 samples and a testing subset with 1,449 samples, all of which have pixel-wise annotations.

    \item \textbf{PASCAL Content~\cite{mottaghi2014role}:} PASCAL Content is an extension of PASCAL VOC 2010 detection dataset~\cite{everingham2010pascal}, which contains more than 400 categories with pixel-wise annotations. It has 4,998 training images and 1,449 validation images.

    \item \textbf{Cityscapes~\cite{cordts2016cityscapes}:} Cityscapes is a dataset for the visual recognition of street scenes. This dataset includes a training subset with 2,975 samples and a testing subset with 500 samples, all of which are with pixel-wise annotations of 19 categories.

\end{itemize}

\subsection*{C.4. Datasets for Object Detection}

\begin{itemize}

    \item \textbf{MS COCO~\cite{lin2014microsoft}:} MS COCO Dataset is a dataset for object detection. It consists of two versions: MS COCO 2014 contains 83,000 training images and 41,000 validation images with bounding box annotations of 80 categories, and MS COCO 2017 contains 118,000 training images and 5,000 validation images with bounding box annotations of 80 categories.

    \item \textbf{ODinW~\cite{li2022elevater}:} ODinW is a benchmark to evaluate the task-level transfer ability of pre-trained vision models, which consists of 35 free public Object Detection datasets in various domains. The dataset contains 132k training images and 20K testing images belonging to 314 concepts. Also, many of the 35 tasks have very limited (fewer than 100) training images, which makes it extremely difficult for standard detectors without any pre-training.
    
    \item \textbf{LVIS~\cite{gupta2019lvis}:} LVIS is a large vocabulary dataset for long-tailed instance detection/ segmentation. The dataset contains 1203 categories with federated human annotations on 100K images.

\end{itemize}

\subsection*{C.5. Datasets for Image and Text Retrieval}

\begin{itemize}

    \item \textbf{Flickr30k~\cite{young2014image}:} Flickr30K is a dataset for automatic image description and grounded language understanding. It contains 31,000 images collected from Flickr, where each image is provided with 5 captions.

    \item \textbf{COCO Caption~\cite{chen2015microsoft}:} COCO Caption contains over 330k images from MS COCO~\cite{lin2014microsoft}. It has two versions: COCO Caption c5 with 5 reference captions for 330k images and COCO Caption c40 that provides 40 reference captions for a randomly sampled subset of 5,000 images.

\end{itemize}
